# Supplementary material for: Quorum Subsumption for Heterogeneous Quorum Systems
Source: arXiv:2304.04979 source file (2023-08-11)
Supplement: Supplementary file 1 [file Appendix.tex]

% \section{Appendix}
{\Huge\!\!\!Appendix}

\tableofcontents

\clearpage
\section{Byzantine Reliable Broadcast}
\subsection{Proofs}
\label{sec:brb-proofs}

\begin{theorem}
\label{thm:quorum-based-rb-suffi-app}
Quorum intersection and strong availability are sufficient to implement Byzantine reliable broadcast.
\end{theorem}

This theorem follows from the following five lemmas.
In the following lemmas, we consider a quorum system with quorum intersection and strong availability for $P$.

% \ec{All the following proofs use proof by contradiction.}

%\textbf{Consistency}
\begin{lemma}
    The BRB protocol guarantees consistency.
%     for well-behaved processes.
\end{lemma}

\begin{proof}
   A well-behaved process only delivers a message when it receives a quorum of consistent ready messages.
   If $p_1$ delivers $m_1$ with $q_1$, and $p_2$ delivers $m_2$ with $q_2$,
   by quorum intersection, there is well-behaved process $p$ in $q_1 \cap q_2$.
   The process $p$ sends ready messages with only one value. Thus, $m_1 = m_2$.
%    
   %Because our quorum system has at least a well-behaved process in the intersection of any pair of quourms.
%    
%    \ec{
%     Suppose two well-behaved processes, $p_1$ and $p_2$, 
%     deliver two different values $v_1$ and $v_2$, respectively, 
%     towards contradiction.
%     If $p_1$ delivered $v_1$, then it must have received a quorum $q_1$ of consistent ready messages for $v_1$.
%     Likewise for $p_2$ and $v_2$ for some quorum $q_2$.
%     By quorum intersection, $q_1$ and $q_2$ must intersect at at least one well-behaved process.
%     However, a well-behaved process readies a value at most once during the protocol, meaning $v_1 = v_2$, 
%     contradicting the assumption that the values differ.
%     }
%    
\end{proof}

\input{BRBValidity}

% \xl{strictly weaker than FBQS}
% \ml{You want to add something here?}
    
%\textbf{Totality}
\begin{lemma}
%     If the quorum system $\Q$ is available for $P$, then 
    The BRB protocol guarantees totality for $P$.
\end{lemma}

\begin{proof}
    We assume that a well-behaved process $p$ has delivered $m$, 
    and show that every well-behaved process $p' ∈ P$ delivers $m$.
    We first show that every well-behaved process $p''$ sends ready messages for $m$
    to its followers.

    The well-behaved process $p$ delivers $m$ only when 
    it receives a quorum $q$ of ready messages for $m$.
%
%     \cap \W
%     $\forall p' \in \W, \forall q' \in \Q(p'), q \cap q' \cap \W \neq \emptyset$.
% 
    Consider a quorum $q''_i$ of $p''$.
    By quorum intersection, $q$ and $q''_i$ intersect in at least a well-behaved process $p_i$.
%     Let $I_i$ be the intersection of the well-behaved processes of $q$,
%     and $q''_i$.
%     Consider an arbitrary process $p_i$ in $I_i$.
%     By quorum intersection,
%     $q$ and $q''$ intersect at a well-behaved process $p_i$.
%     Consider a process $p_i$ in the intersection of well-behaved processes of $q$, and $q''$.
    Since $p_i$ is in $q''_i$, 
%     then $p''$ is a follower of $p_i$.
    then $p_i$ has $p''$ as a follower.
%
%     All well-behaved processes in $q$ send ready messages to their followers including $p''$.
%     All well-behaved processes in $q$ send ready messages to their followers.
%     Thus, $p_i$ sends a ready message to $p''$.
%     Thus, $p_i$ sends a ready message to $p''$.
%
    Let $I$ be the union of the processes $p_i$ for all quorums $q''_i$ of $p''$.
    By construction,
    the set of processes $I$ are a subset of $q$, a blocking set of $p''$, and have $p''$ as a follower.
%     $p''$ is a follower of it.
%     
%     By quorum intersection,
%     $q$ intersects all quorums in the system in at least one well-behaved process.
%
%     Therefore, 
% %     for any well-behaved process $p'$, 
%     well-behaved processes of $q$ are $p''$-blocking.
% 
%    Since all processes in $q$ have broadcast ready messages,
   All well-behaved processes in $q$ send ready messages to their followers.
   Thus, the set of processes $I$ send ready messages to $p''$.
   Thus, $p''$ receives a blocking set of ready messages,
   and sends ready messages to its followers.
%     The well-behaved process $p'$ has a quorum $q'$ with all well-behaved members.

   Thus, every well-behaved process $p''$ sends ready messages to their followers.
   By weak availability, $p' \in P$ has a quorum $q'$ with all well-behaved members.   
   Thus, the process $p'$ will receive ready messages from $q'$, and delivers $m$.
% 
%     \ml{Eric, the following proof looks good. It is just that direct proofs are more natural than proofs by contradiction. I took parts of the proof below to the direct proof above.}
% 
%     \ec{
%     Suppose a well-behaved process $r$ delivers a message, 
%     but there is some process $p \in P$ that does not deliver a message, towards contradiction.
%     Since the quorum system is strongly available for $P$, and $p \in P$,
%     $p$ has at least one complete quorum $q_p$.
%     If $p$ does not deliver a message, it never receives any quorum of consistent ready messages.
%     This means at least one process in $q_p$ does not send a ready message to $p$.
%     Let this process be $p'$.
%     If (well-behaved) $p'$ does not send a ready message to $p$,
%     it did not receive a blocking set of consistent ready messages (nor a quorum of consistent echo messages).
%     }
%     
%     \ec{
%     Since $r$ delivers a message,
%     it must have received a quorum $q_r$ of consistent ready messages.
%     By quorum intersection, for every quorum of $p'$, it intersects $q_r$ at at least one well-behaved process.
%     That is, $q_r \cap \W$ is a blocking set for $p'$.
%     Then, if every well-behaved process in $q_r$ sent a ready message to $r$, then it must also have sent a ready message to $p'$.
%     However, this means $p'$ would have received a blocking set of consistent ready messages,
%     thus reaching a contradiction.
%     }    
\end{proof}

% \ec{
% im missing the reasoning here, how does $p'$ sending ready to its followers 
% imply that every member in $q''$ of $p''$ receives ready?
% }

%\textbf{No duplication}

\begin{lemma}
   The BRB protocol guarantees no duplication.
%     for all the well-behaved processes.
\end{lemma}

\begin{proof}
Since a well-behaved process keeps the $\mathit{delivered}$ boolean,
it delivers at most one message.
%     A well-behaved process delivers a message $m$ only when it receives a quorum of ready messages for $m$. By quorum intersection, every pair of quorums intersect at a well-behaved process. A well-behaved process keeps the $\mathit{readied}$ boolean and only sends out ready messages for one $m$. Therefore, a well-behaved process cannot deliver 
\end{proof}

% \textbf{Integrity}

\begin{lemma}
   The BRB protocol guarantees integrity.
%     for all the well-behaved processes.
\end{lemma}

\begin{proof}
    We assume that a well-behaved process $p$ delivers a message $m$ from a well-behaved sender process $p'$,
    and prove that the process $p'$ has broadcast $m$.     
    We first prove that 
    a well-behaved process has received echo messages from at least one of its quorums.

    Since the well-behaved process $p$ delivered $m$, 
    it has received a quorum $q_p$ of ready messages.
    By the strong availability assumption, 
    $P$ is non-empty; therefore,
%     \ec{This is only true if $P$ is non-empty, which is strange since integrity is not qualified by $P$. 
%     Also, $P$ can technically be empty for all the other properties.
%     Maybe something about non-trivial?
%     }
    there exists a process 
%     $p$ 
    with a quorum $q$ that is well-behaved and quorum subsuming.
    By quorum intersection, 
%     $q \cap q_r \cap \W \neq \emptyset$.
    $q_p$ and $q$ intersect at a well-behaved process $p_i$.
%     Let $p_i$ be a member of $q \cap q_r \cap \W$ which sent the ready message.
    The process $p_i$ sent a ready message (that $p$ received).
    The well-behaved process $p_i$ sends a ready message only if it
    either (1) receives echo messages from a quorum of $p_i$, 
    or (2) receives ready messages from a $p_i$-blocking set $B$.
    The first case is immediately the conclusion with the process $p_i$.
    Let us consider the second case.
    By quorum subsumption, 
    since $p_i$ is in $q$, 
    $p_i$ has a quorum $q_i$ that is a subset of $q$.
    Since $B$ is a blocking set of $p_i$,
    $B$ intersects with $q_i$.
    Therefore, $B$ intersects with $q$.
%     $\exists q_i \in \Q(p_i), q_i \subseteq q \subseteq \W \wedge b \cap q_i \neq \emptyset$.  
   The processes in $B$ sent ready messages.
   Thus, there are processes in $q$ that sent ready messages.
   Let $p_f$ be the first process in $q$ that sent a ready message.
   All members of $q$ are well-behaved.
    A well-behaved process $p_f$ sends a ready message only if it
    either (1) receives echo messages from a quorum of $p_f$, 
    or (2) receives ready messages from a $p_f$-blocking set $B'$.
    The first case is immediately the conclusion with the process $p_f$.
    Let us consider the second case.   
    Applying the same reasoning as for $p_i$ to $p_f$
    derives that $B'$ intersects with $q$.
    Thus, $p_f$ has received a ready message from a process in $q$.
    Therefore, $p_f$ is not the first process in $q$ to send a ready message.
    This is a contradiction with the definition of $p_f$ above.

    We now use the fact that 
    a well-behaved process has received echo messages from at least one of its quorums.
   By quorum intersection at well-behaved processes,
   every quorum of a well-behaved process includes a well-behaved process.
   %Then the first ready message is sent by receiving a quorum of echo messages.
%    Since every quorum of a well-behaved process includes itself,    
%    $q_e$ includes $p_e$.
%     
%     Therefore, $p_e$ has received an echo message from itself.
   Thus, a well-behaved process $p_w$ has sent an echo message.
    A well-behaved process sends an echo message only after receiving it from the sender $p'$.
    Since the sender $p'$ is well-behaved,
    and $p_w$ has received the message $m$ from it,
    by the integrity of point-to-point links,
    $p'$ has previously sent $m$ to $p_w$.
    Since $p'$ is well-behaved, 
    it has sent $m$ to every process.
%
%     \ec{
%     Suppose a well-behaved process $r$ delivers a message $m$ and the sender is well-behaved, 
%     but the sender did not previously broadcast $m$, towards contradiction.
%     If $r$ delivers $m$, then it received a quorum $q_r$ of consistent ready messages.
%     }
%     
%     \ec{
%     Let $p \in P$.
%     Let $q_p$ be the complete quorum of $p$.
%     By quorum intersection, there is a well-behaved process $p_i \in q_p \cap q_r$.
%     If $p_i$ sent a ready message to $r$,
%     then one of the following must be true:
%     (1) $p_i$ received a quorum of consistent echo messages, or
%     (2) $p_i$ received a $p_i$-blocking set of consistent ready messages.
%     }
% 
%     \ec{
%     In the first case, 
%     since every quorum of $p_i$ contains itself,
%     $p_i$ sent an echo message (to itself).
%     However, a well-behaved process only sends an echo message upon receiving a message from the sender,
%     contradicting the assumption that the sender did not broadcast $m$.
%     }
% 
%     \ec{
%     In the second case,
%     $p_i$ received a $p_i$-blocking set of consistent ready messages.
%     (Can you just do $p_f$ here as well?)
%     }
\end{proof}

\clearpage
\section{Byzantine Consensus}
\subsection{Proofs}
\label{sec:consensus-proofs}

\begin{theorem}
   \label{thm:quorum-based-c-suffi-app}
   Quorum intersection and strong availability are sufficient to implement consensus.
\end{theorem}

This theorem follows from the following three lemmas
where
% 	In the following lemmas, 
we consider a quorum system with quorum intersection and strong availability for $P$.

%\textbf{Agreement}
\begin{lemma}[Agreement]
   The consensus protocol guarantees agreement.
%    for well-behaved processes.
\end{lemma}

\begin{proof}   
   We prove agreement by contradiction.
   Assume that there are two well-behaved processes that decide two different values.
   A process decides a value at \autoref{algC:decision-reponse} after delivering a ballot with that value at \autoref{algC:commit-prepared}.
   Let process $p$ deliver $v$ in ballot $b$, and let process $p'$ deliver $v'$ in ballot $b'$.
   Since ballots are totally ordered, without loss of generality, we assume that $b ⋦ b'$.
   When the process $p'$ delivers $v'$ at \autoref{algC:commit-prepared}, 
   it checks that $b'$ has been prepared.
   A well-behaved process prepares a new ballot $b'$ at \autoref{algC:update-prepared}
   only after finding all the ballots below and incompatible with $b'$ aborted at \autoref{algC:prepared}.
   Since $b ⋦ b'$, the process $p'$ 
%    finds $b$ aborted 
   has delivered the $\mathbb{A}$ message for $b$
   before preparing $b'$.
%    is prepared.
   However, since process $p$ decides $v$ with $b$ at \autoref{algC:decision-reponse}, 
   it has delivered $\mathbb{C}$ message for $b$
   at \autoref{algC:commit-prepared}.
   Thus, two well-behaved processes deliver conflicting values $\mathbb{A}$ and $\mathbb{C}$ for ballot $b$, which violates the consistency property of federated voting, a contradiction.
\end{proof}

% \xl{stronger than abstarct consensus}

%\textbf{Weak validity}
% \begin{lemma}[Weak validity]
\begin{lemma}[Validity]
%    The consensus protocol guarantees weak validity for well-behaved processes.
   The consensus protocol guarantees validity.
%    for well-behaved processes.
\end{lemma}

\begin{proof}
%    ((Weak) validity).        
%    If all processes are well-behaved and propose the same value, 
%    then no well-behaved process decides a different value;
%    furthermore, if all processes are well-behaved, and some process decides a value, 
%    then that value was proposed by some process.
% 
% 
%          (Validity).
%          If all processes are well-behaved, and some process decides a value, 
%          then that value was proposed by some process.
% 
%
   We assume that all processes are correct,
   and that a process has decided a value $v$.
   We show that $v$ is proposed by some process.
   When a well-behaved process decides a value $v$ at \autoref{algC:decision-reponse}, 
   $v$ was delivered in a $\mathbb{C}$ message for a ballot $b$ 
%    and $b.v = v$
   at \autoref{algC:commit-prepared}.
   Since all processes are well-behaved including the leader, by the integrity property of federated voting,
   the leader has broadcast $\mathbb{C}$ for the ballot $b$ at \autoref{algC:leader-commit}.
   The ballot $b$ is the leader's $\candidate$ by the condition at \autoref{algC:prepare-candidate}.
   
   We show that the value of every $\candidate$ ballot can be tracked back to the proposal of a process.   
   The value for the $\candidate$ ballot is set to either its initial proposal at \autoref{algC:assign-proposal} and \autoref{algC:update-candidate-default}, 
   or adopted from the value of $\prepared$ at \autoref{algC:update-candidate}.
   We consider the two cases in turn.
   For the first case, the value $v$ is immediately the leader's proposal at \autoref{algC:propose}.   
%    If all the processes are well-behaved, then $v$ was proposed by some well-behaved process, which is the leader.
%    
   For the second case, $v$ is a value prepared before by the leader.
   A well-behaved process updates its $\prepared$ value to $b$ at \autoref{algC:update-prepared}
   when it delivers $\mathbb{A}$ for all $b' ⋦ b$ at \autoref{algC:prepared}.
   By the integrity of federated voting, and the assumption that all the processes are well-behaved, 
%    other processes 
   leaders have broadcast to abort all ballots $b'$.
   Leaders abort ballots below and incompatible with their $\candidate$
   at \autoref{algC:leader-abort} and \autoref{algC:abort-new-round}.
   By the batched network semantics assumption, 
   all the messages sent by a process in one event to another process are delivered and processed together.
   Therefore, the ballot $b$ has been the $\candidate$ ballot of a previous leader
   at \autoref{algC:leader-abort} or \autoref{algC:abort-new-round}.
   With the same reasoning as above,
   the $\candidate$ value can be traced back to either
   a proposal, or the $\candidate$ value of a yet previous leader.
   Since the number of leaders is finite, 
   by a well-founded induction,
%    Therefore, by induction,
%    the value of $b$ has been the proposal of a process.
   the $\candidate$ value is tracked back to the proposal of a process.
%    By induction for the $\prepared$ value, 
%    the first $\prepared$ ballot (excluding the default $\angled{0, \bot}$) at a well-behaved process is due to some leader using BRB to abort for its $\candidate$ with its initial proposal (at \autoref{algC:assign-proposal} and \autoref{algC:update-candidate-default}).
%    Then $v$ was proposed by that leader.
% 
\end{proof}

   The protocol guarantees termination:
% 	regardless of Byzantine behavior, 
	all strongly available processes eventually decide a value.
	The high-level idea is that 
	by eventual election of a well-behaved leader,
% 	by 
   and
	the totality property of federated voting,
% 	and eventual leader election module, 
% 	a well-behaved leader eventually prepares the highest ballot that is prepared at any well-behaved process in the system.
	a well-behaved leader eventually adopts the value of the highest prepared ballot in the system as its candidate
% 	Then, that leader can proceed to commit that ballot.
	Then, that leader can proceed to prepare and commit its candidate.
% 	with the abort and commit process with BRB 
% 	will be accepted by all the strongly available processes.

%\textbf{Weak liveness}
\begin{lemma}[Termination]
% If the quorum system $\Q$ is strongly available for $P$, then 
The consensus protocol guarantees termination for $P$.
\end{lemma}

\begin{proof}
The proof will refer to the notions of locked for federated voting.
We first visit these notions, and then describe the proof of termination.

We saw in the explanation of the protocol that
there are executions that Byzantine processes can lock a federated voting instance
for a certain value (such as commit).
Let us remember that example.
Consider that we have 4 processes, one of them is Byzantine,
and any set of 3 processes is a quorum.
Let the Byzantine process send a message $m$ to one well-behaved process.
That well-behaved process echos $m$.
% However, a well-behaved process has already echoed commit,
If the Byzantine process remains silent,
the remaining 2 well-behaved processes are not a quorum,
and even if both echo another message $m'$,
they cannot make the federated voting deliver $m'$.
This execution is shown in the first two rounds of messages in \autoref{fig:proof-fig}.
In this execution, the federated voting instance of $b$ is locked for $m = \mathbb{C}$ by $l₁$ and $p₃$,
and
although $l₂$ and $p₄$ try to make it deliver $m' = \mathbb{A}$, it does not.
However, if the Byzantine process echos $m'$ as well,
then they form a quorum, and can make $m'$ be delivered.
Well-behaved processes alone cannot make the instance deliver a different value,
but well-behaved and Byzantine processes together can.
We call these states of the federated voting abstraction soft-locked.

We note that 
there are also states of a federated voting instance where
even if well-behaved and Byzantine processes 
work together, they cannot make the instance deliver a different value.
We call them hard-locked.
% We first note that
% after certain steps,
% a federated voting instance can get locked for a certain value.
%
As above,
% consider an execution of federated voting where 
% a blocking set of a process $p$ in $P$ echos a message $m$.
% The process $p$ cannot deliver any message other than $m$.
% If 
consider an execution with 4 processes,
% and a Byzantine sender,
and quorums of size 3.
Let a Byzantine process send $m$ to two well-behaved processes, and make them echo $m$.
% sender sends the message $m$ to two of the process and they 
By the protocol,
in order to deliver a message, a process needs to receive at least three ready messages.
Further,
in order to send a ready message, a process needs to receive
at least either
three echo messages
or
two ready messages.
Therefore, to deliver any other message $m'$, 
at least 3 processes should echo $m'$.
Since 2 well-behaved processes out of 4 processes already echoed $m$, and
well-behaved processes echo only once,
there are not 3 processes to echo $m'$,
and make it delivered.
% the message $m'$ cannot be delivered.
% 
The federated voting abstraction is hard-locked for $m$.

% a well-behaved process 
% For example, 
% as we saw in the proof of consistency of BRB,
% a process can deliver a message $m$ if 
% then no well-behaved process $p'$ can deliver another message $m'$.
% This is because
% the fact that $p$ sent ready $m$
% can be tracked back to 
% the fact that some well-behaved process received echo message from one of its quorums $q$.
% Because of quorum intersection,
% a well-behaved process $p$ sends ready messages for $m$,

We now consider the proof of termination.
By the eventual leader election,
there will eventually be a well-behaved leader with a long enough timeout.
Let $b$ be the $\candidate$ ballot of the leader.
The leader tries to abort all ballots lower and incompatible with $b$
at
\autoref{algC:leader-abort}
and
\autoref{algC:abort-new-round}.
We consider three cases based on whether
there is a ballot $b' ⋦ b$ that
% $ below and incompatible with $
% is either committed or is locked for commit.
is locked for commit.
% (We say that a ballot is committed if a well-behaved process has delivered commit for that ballot.)

Case 1:
There is no such ballot $b'$.
The leader can abort all ballots below and incompatible with $b$
at \autoref{algC:prepared},
and broadcast commit for $b$
at \autoref{algC:leader-commit}.
By the validity of federated voting,
all processes in $P$ eventually deliver commit for $b$
at \autoref{algC:commit-prepared},
and decide its value
at \autoref{algC:decision-reponse}.

Case 2:
There is such a ballot $b'$ that is soft-locked for commit.
% but 
% Byzantine and well-behaved processes together can make the instance deliver abort.
%
In order to prepare $b$,
the leader tries to abort $b'$.
If the Byzantine processes cooperate,
it can abort $b'$ and prepare $b$
at \autoref{algC:prepared}, 
and broadcast commit for $b$
at \autoref{algC:leader-commit}.
However, if the Byzantine processes do not cooperate,
the leader cannot abort $b'$.
Therefore, the leader does not succeed, and the timeout is triggered.
Eventually, a well-behaved process $l$ will be the leader.
Since the delay $Δ$ is larger than the bounded communication delay after GST,
% The delay $Δ$ for the leader $l'$ helps him to observe the highest prepared ballot $b$,
the leader $l$ observes the highest prepared ballot $b$
at \autoref{algC:prepared},
and adopts its value as the value of its $\candidate$ $b'$
at \autoref{algC:prepare-candidate}.
We note that when it tries to prepare $b'$, 
since $b'$ is compatible with $b$, it does not need to abort $b$.
Therefore, it can prepare and broadcast commit for $b'$
at \autoref{algC:leader-commit}.
% and decide.
By the validity of federated voting,
all processes in $P$ eventually deliver commit for $b'$
at \autoref{algC:commit-prepared},
and decide its value
at \autoref{algC:decision-reponse}.

Case 3:
There is such a ballot $b'$ that is hard-locked for commit.
% but 
% even Byzantine and well-behaved processes together cannot make the instance deliver abort.
% 
% By the consistency of federated voting, 
Ballot $b'$ cannot be aborted.
Therefore,
% no well-behaved leader 
no well-behaved process can prepare 
% and try to commit 
a ballot with a value incompatible with $b'$.
The current leader will eventually timeout.
Further, all ballots $b'' ⋦ b'$ should have been aborted
since processes accept commit for $b'$ only if $b'$ is $\prepared$
at \autoref{algC:commit-prepared}.
By the totality of federated voting,
eventually a well-behaved leader that has delivered abort for all ballots $b''$
% below and incompatible with $b'$
will be elected.
Therefore, that leader finds $b'$ prepared
at \autoref{algC:prepared}-\ref{algC:update-prepared}, and 
adopts its value as the value of its $\candidate$ ballot $b₂''$
at \autoref{algC:update-candidate}.
Thus, $b₂''$ is compatible with $b'$.
As we saw above,
% any prepared ballot larger than $b'$ is compatible with $b'$
no ballot incompatible with $b'$ can be prepared.
Thus, no ballot incompatible with $b₂''$ can be prepared.
% The candidate of that leader
Thus, the leader can successfully prepare $b₂''$ 
at \autoref{algC:prepared}, 
and broadcast commit for $b₂''$
at \autoref{algC:leader-commit}-\ref{algC:prepare-candidate}.
By the validity of federated voting,
all processes in $P$ eventually deliver commit for $b₂''$
at \autoref{algC:commit-prepared},
and decide its value
at \autoref{algC:decision-reponse}.
\end{proof}

\clearpage
\subsection{Example Execution}
\label{sec:example-execution}

We demonstrate an execution of our consensus protocol, which illustrates its ability to fulfill both safety and liveness properties.
Let us assume $\P = \{1, 2, 3, 4\}, \B = \{2\}, \Q(1) = \{\{1, 2, 3 \}\}, \Q(3) = \{\{3, 4\}, \{1, 3\}\}, \Q(4) = \{\{3, 4\}\}$.
All the well-behaved processes are initialized with a default ballot $\angled{0, \bot}$ for their $\prepared$ and $\candidate$ variable.
The well-behaved processes propose three different values: process $1$ propose $3$; process $3$ propose $5$; process $4$ propose $2$.

In the first round, process $1$ is the leader.
Upon the proposal at \autoref{algC:propose}, all the well-behaved process update their $\candidate$ with their own proposal value at \autoref{algC:assign-proposal}.
Process $1$ aborts all the ballots below and incompatible with its $\candidate$ through reliable broadcast: it $\mathit{BCast} \mathbb{A}$ for instances $\angled{0, \bot}$, $\angled{1, 1}$ and $\angled{1, 2}$ at \autoref{algC:leader-abort}.
Since the network is partially synchronized, we let the process $4$ be partitioned from the rest of processes temporarily.
Byzantine process $2$ only send $\mathit{Echo} \mathbb{A}$ messages for ballot $\angled{0, \bot}$ and $\angled{1, 1}$.
Since process $1$ has the individual minimal quorum $\{1, 2, 3\}$, it send $\mathit{Ready} \mathbb{A}$ messages for the aforementioned two ballots.
Process $3$ sends $\mathit{Ready} \mathbb{A}$ messages for the two ballots, too.
We partition process $3$ from process $1$ and $2$ from now on temporarily.
Process $1$ is able to deliver the $\mathbb{A}$ for ballots $\angled{0, \bot}$ and $\angled{1, 1}$ through BRB at \autoref{algC:prepared} and update its $\prepared$ variable as $\angled{1, 2}$ at \autoref{algC:update-prepared}.
Since the leader process $1$'s $\prepared \neq \candidate$, it can not broadcast commit for its $\candidate$ and the timer triggers.

In the second round, Byzantine process $2$ is the leader.
When the new leader is elected for a new round, all the well-behaved process increase their round number and update their $\candidate$: process $1$ updates its $\candidate$ value to its prepared value $2$ at \autoref{algC:update-candidate};
process $3$ and $4$ has not prepared any ballot and update their candidate to their original proposal at \autoref{algC:update-candidate-default}.
Then Byzantine leader tries to commit an arbitrary value $4$, which no well-behaved process will accept, since the well-behaved process only deliver $\mathbb{C}$ for a BRB instance with the ballot same as its $\prepared$ at \autoref{algC:commit-prepared}.
We recovery the connection from process $3$ and $4$ to the rest of the network.
Then both process $3$ and $4$ delivers $\mathbb{A}$ message from previous round at \autoref{algC:prepared} and update their $\prepared$ ballot to $\angled{1, 2}$.
No value is decided and the timer trigger again.

In the third round, well-behaved process $3$ is the leader.
All the well-behaved process now synchronized to the same highest prepared ballot $\angled{1, 2}$ and update their $\candidate$ accordingly.
Process $3$ then abort the rest ballots that are less and incompatible with its $\candidate = \angled{3, 2}$ through BRB.
Byzantine process $2$ remain silent in this round to prevent liveness for the weakly available process $1$.
However, process $3$ and $4$ are strongly available and is able to successfully deliver the abort messages.
Their $\prepared$ is updated to $\angled{3, 2}$ and process $3$ commits this ballot through BRB at \autoref{algC:leader-commit}.
All the process $3$ and $4$ deliver the commit message at \autoref{algC:commit-prepared} and decide the value $2$ in the committed ballot $\angled{3, 2}$ at \autoref{algC:decision-reponse}.

\begin{table*}[h!]
	\small
	% 	\scalebox{0.7}{
		% 	\hspace*{-1.7cm}
		\centering
		% 	\begin{tabular}{|c @{} c @{} c @{} c|} 
			\begin{tabular}{|c c c c|} 
				\hline
				1 & \textcolor{red}{2} & 3 & 4 \\ 
				\hline
				$p = \angled{0, \bot}$&  & $p = \angled{0, \bot}$ & $p = \angled{0, \bot}$ \\ 
				$c = \angled{0, \bot}$& & $c = \angled{0, \bot}$ & $c = \angled{0, \bot}$ \\ 
				\hline
				$\mathit{Propose(3)}$ &  & $\mathit{Propose(5)}$ & $\mathit{Propose(2)}$\\
				\hline
				$p = \angled{0, \bot}$&  & $p = \angled{0, \bot}$ & $p = \angled{0, \bot}$ \\ 
				$c = \angled{1, 3}$& & $c = \angled{1, 5}$ & $c = \angled{1, 2}$ \\ 
				\hline
				$\mathit{BCast(\angled{0, \bot}, Abort)}$ &  & & \\
				$\mathit{BCast(\angled{1, 1}, Abort)}$ &  & & \\
				$\mathit{BCast(\angled{1, 2}, Abort)}$ &  & & \\
				\hline
				$\mathit{Echo(\angled{0, \bot}, Abort)}$& \textcolor{red}{$\mathit{Echo(\angled{0, \bot}, Abort)}$} & $\mathit{Echo(\angled{0, \bot}, Abort)}$& slow \\
				$\mathit{Echo(\angled{1, 1}, Abort)}$& \textcolor{red}{$\mathit{Echo(\angled{1, 1}, Abort)}$} & $\mathit{Echo(\angled{1, 1}, Abort)}$&  \\
				$\mathit{Echo(\angled{1, 2}, Abort)}$& & $\mathit{Echo(\angled{1, 2}, Abort)}$&  \\
				\hline
				$\mathit{Ready(\angled{0, \bot}, Abort)}$ & $\textcolor{red}{\mathit{Ready(\angled{0, \bot}, Abort)}}$ & $\mathit{Ready(\angled{0, \bot}, Abort)}$ & slow\\
				$\mathit{Ready(\angled{1, 1}, Abort)}$ & $\textcolor{red}{\mathit{Ready(\angled{1, 1}, Abort)}}$ & $\mathit{Ready(\angled{1, 1}, Abort)}$ & \\
				\hline
				$\mathit{Deliver(\angled{0, \bot}, Abort)}$ &  & slow & slow \\ 
				$\mathit{Deliver(\angled{1, 1}, Abort)}$ &  &  & \\ 
				\hline
				$p = \angled{1, 2}$&  & $p = \angled{0, \bot}$ & $p = \angled{0, \bot}$ \\ 
				$c = \angled{1, 3}$&  & $c = \angled{0, \bot}$ & $c = \angled{0, \bot}$ \\ 
				\hline
				time out & & time out & time out \\
				\hline
				$p = \angled{1, 2}$&  & $p = \angled{0, \bot}$ & $p = \angled{0, \bot}$ \\ 
				$c = \angled{2, 2}$&  & $c = \angled{2, 5}$ & $c = \angled{2, 2}$ \\ 
				\hline
				&  \textcolor{red}{$\mathit{BCast(\angled{2, 4}, Commit)}$}& & \\
				\hline
				& & $\mathit{Deliver(\angled{0, \bot}, Abort)}$ & $\mathit{Echo(\angled{0, \bot}, Abort)}$ \\
				&  & $\mathit{Deliver(\angled{1, 1}, Abort)}$ & $\mathit{Echo(\angled{1, 1}, Abort)}$ \\
				& & & $\mathit{Echo(\angled{1, 2}, Abort)}$ \\
				& & & $\mathit{Ready(\angled{0, \bot}, Abort)}$ \\
				& & & $\mathit{Ready(\angled{1, 1}, Abort)}$ \\
				& & & $\mathit{Delivery(\angled{0, \bot}, Abort)}$ \\
				& & & $\mathit{Delivery(\angled{1, 1}, Abort)}$ \\
				\hline
				$p = \angled{1, 2}$&  & $p = \angled{1, 2}$ & $p = \angled{1, 2}$ \\ 
				$c = \angled{2, 2}$&  & $c = \angled{2, 5}$ & $c = \angled{2, 2}$ \\ 
				\hline
				time out & & time out & time out \\
				\hline
				$p = \angled{1, 2}$&  & $p = \angled{1, 2}$ & $p = \angled{1, 2}$ \\ 
				$c = \angled{3, 2}$&  & $c = \angled{3, 2}$ & $c = \angled{3, 2}$ \\ 
				\hline
				& & $\mathit{BCast(\angled{1, 2}, Abort)}$ ...& \\
				\hline
				& silent &$\mathit{Deliver(\angled{1, 2}, Abort)}$... &$\mathit{Deliver(\angled{1, 2}, Abort)}$... \\
				\hline 
				$p = \angled{1, 2}$&  & $p = \angled{3, 2}$ & $p = \angled{3, 2}$ \\ 
				$c = \angled{3, 2}$&  & $c = \angled{3, 2}$ & $c = \angled{3, 2}$ \\ 
				\hline
				& & $\mathit{BCast(\angled{3, 2}, Commit)}$ & \\
				\hline
				& silent &$\mathit{Deliver(\angled{3, 2}, Commit)}$ &$\mathit{Deliver(\angled{3, 2}, Commit)}$ \\
				\hline
				& silent & \textcolor{green}{$\mathit{Decide(2)}$} & \textcolor{green}{$\mathit{Decide(2)}$} \\
				\hline
			\end{tabular}
			% 	}
		\caption{An execution for consensus protocol with leader switch }
		\label{table:consensus-changeleader}
	\end{table*}

\clearpage
\section{Discussion}
\label{sec:discussion}

When Byzantine processes don't lie about their slices,
an FBQS 
% The Federated Byzantine quorum system 
enjoys quorum sharing \cite{losa2019stellar}.
% (A similar observation is made about PBQSs \cite{losa2019stellar}.)
% ☞{This is proof for quorum sharing not quorum subsumption?}
% 
% By the protocol above,
Consider a quorum $q$ of a process $p$, and a process $p'$ in it.
Since 
a set is recognized as a quorum only if it contains a slice for each of its members,
the process 
$p'$ has a slice $s$ in $q$.
Processes receive the same set of slices from a given process even if it is Byzantine.
If $p'$ starts from $s$, 
it can find a quorum that grows no larger than $q$,
\ie, it can stop at $q$ if not earlier.
Therefore, $q$ includes a quorum of $p'$.

However, when Byzantine processes lie about their slices, FBQS does not satisfy quorum sharing.
Consider an FBQS with five processes 
$\P = \{1, 2, 3, 4, 5\}$,
and one Byzantine process $𝓑 = \{ 4 \}$.
The slices of well-behaved processes $\W = \{1, 2, 3, 5\}$ are the following: $\S(1) = \{\{1, 2\}\}$, $\S(2) = \{\{2, 3\}, \{2, 4\}, \{2, 5\}\}$, $\S(3) = \{\{3, 4\}\}$, $\S(5) = \{\{2, 5\}\}$.
However, the Byzantine process $4$ provides different quorum slices to different well-behaved processes. 
The slices that it sends to each other process are the following: $\S(4)_1 = \{\{1, 4\}\}$, $\S(4)_2 = \{\{3, 4\}\}$, $\S(4)_3 = \{\{2, 4\}\}$, $\S(4)_5 = \{\{4, 5\}\}$.
By the definition of quorums in FBQS, 
% and the local view of each process
we have the following individual minimal quorums for each well-behaved process:
$\Q(1) = \{\{1, 2, 4\}, \{1, 2, 5\}\}$, $\Q(2) = \{\{2, 3, 4\}, \{2, 5\}\}$, $\Q(3) = \{\{2, 3, 4\}\}$, $\Q(5)$ $=$ $\{\{2, 5\}\}$.
We can see that $\Q$ does not have quorum sharing,
since the quorum $\{1, 2, 4\}$ does not include any quorum for process $2$.
However, $\Q$ is strongly available for processes $\{1, 2, 5\}$,
since they all have quorums that are well-behaved and quorum subsuming.
Notice that abstract quorums which are over-approximations of FBQS satisfy quorum-sharing \cite{losa2019stellar}: A set $q$ is an abstract quorum of a process $p$ if $p$ is Byzantine, or $p$ has a slice contained in $q$ and every well-behaved member of $q$ has a slice contained in $q$.
However, as shown in our example, not all abstract quorums of a process can be observed by that process when Byzantine processes lie about their quorum slices.
For example, $\{1, 2, 4\}$ is an abstract quorum of process $2$ but $2$ does not observe it when the Byzantine process $4$ lies. 
Therefore, relaxation of the quorum sharing is necessary when analyzing 
quorum systems such as FBQS when Byzantine processes lie.

Further, there are systems where a strongly available set exists but no guild set (from ABQS) exists.
% Therefore, HQS can provide stronger safety and liveness properties than ABQS.
Therefore, HQS can provide safety and liveness for those executions but ABQS cannot.
% 2) The maximal strongly available set (from this work) is a strict superset of a maximal guild (from ABQS):
% ☞{Is this too general to say?}
% 
% All the maximal guilds in ABQS are strongly available in HQS with quorum intersection; however, the opposite is not true.
We show a quorum system that has an empty guild but has non-empty strongly available set and quorum intersection.
Let $\P = \{1, 2, 3, 4\}$, and process $3$ is Byzantine. 
Let the asymmetric failure prone system be $\F(1) = \{\{3, 4\}, \{2\}\}$, $\F(2) = \{\{3, 4\}, \{1\}\}$, $\F(3) = \{\{1, 2\}\}$, $\F(4) = \{\{2, 3\}\}$. 
The canonical quorum systems are $\Q(1) = \{\{1, 2\}, \{1, 3, 4\}\}$, $\Q(2) = \{\{1, 2\}, \{2, 3, 4\}\}$, $\Q(3)= \{\{3, 4\}\}, \Q(4) = \{\{1, 4\}\}$. 
This HQS has quorum intersection and a non-empty strongly available set:
all the quorums of well-behaved processes have at least one correct process in their intersection. 
The set $\{1, 2\}$ is a strongly available set for $\Q$. 
However, it is not an ABQS with generalized $B^3$ condition. 
%However, the condition $B^3$ does not hold. 
For processes $1$ and $2$, $\F_1 = \{2\}, \F_2 = \{1\}$ and $\F_{12} = \{3,4\}$, and we have $\P ⊆ \{2\} \cup \{1\} \cup \{3, 4\}$, which violates generalized $B^3$.
Therefore this quorum system is not an ABQS. There is no guild set.
