# Supplementary material for: Quorum Subsumption for Heterogeneous Quorum Systems
Source: arXiv:2304.04979 source file (2023-08-11)
Supplement: Supplementary file 2 [file AppendixEnd.tex]

\subsection{Reconfiguration protocol for classic DQS}

\textbf{The Primitives for Reconfiguration Service. \ }
Here we define the primitives for reconfiguration service for classic dissemination quorum system. The well-formed reconfiguration request means that after applying the reconfiguration, the quorum system maintains non-empty outlive set.

$\mathbf{Validity:}$ If a well-behaved process proposes a well-formed reconfiguration request, which does not overlapped with other reconfiguration requests, then every well-behaved process eventually completes the reconfiguration request.

$\mathbf{Totality:}$ If a well-behaved process completes a reconfiguration request, then every well-behaved process eventually completes a reconfiguration request.

$\mathbf{Consistency:}$ If some well-behaved process completes a reconfiguration request and the quorum system is updated to $𝓠$, another well-behaved process completes a reconfiguration request and the quorum system is updated to $𝓠'$, then $𝓠 = 𝓠'$.

$\mathbf{Integrity:}$ If the original quorum systems is $𝓠'$ and some well-behaved process completes a reconfiguration request for a resulting quorum system $𝓠$ and the sender process is well-behaved, then $|𝓠 - 𝓠'|$ was previously proposed by the sender.

\textbf{Leave protocol in DQS. \ }
For leave request in the dissemination quorum system, a well-behaved process $v$ first checks whether its absence will leave the quorum intersection with no well-behaved process. If not, the leave request is not well-formed and will be dropped. If the local check passes, $v$ send the leave request to a total order broadcast. When the leave request is delivered to a process $v'$, it will check the quorum intersection property with the absence of process $v$. This second validation is necessary because of concurrent leave requests may appear. At the delivery of process $v$'s leave request from TOB, there is no gurantee that the quorum system stays unchanged as the time leave request was proposed. TOB ensures that all the well-behaved processes have the same quorum systems and the second check's results are consistent. If the second check passes, process $v'$ removes $v$ from all the quorums and completes leave request successfully. If not, the leave request is ignored for safety.

\textbf{Join protocol in DQS. \ }
For join operation in dissemination quorum system, a process $v$ can propose a join request with new quorums $𝓠_{new}$ and failure assumptions $\B_{new}$. Since the new process only knows the current members instead all the quorum configurations, it can only check quorum availability property based on it's own knowledge. Then process $v$ sends its join request with $𝓠_{new}, \B_{new}$ to the total order broadcast. When the join reuqest is delivered at a well-behaved process $v'$, $v'$ checks whether quorum intersection property is satisfied from the combination of the existing quorum system and the new one. Since all the well-behaved processes maintains the same quorum system, the check's results are consistent. If the check pass, $v'$ adds $𝓠_{new}$ and $\B_{new}$ to its quorum system and sends back the updated quorums and failure assumptions to $v$. If $v$ receives a quorum of responses, it can safely initialize its quorums and failure assumptions and the join operation is completed. Note that after a join operation, all the processes including the newly joined process and existing ones keeps a  classic dissemination quorum system with the same quorums and failure assumpions.

\textbf{Delete a quorum in DQS}
When removing a quorum, quorum intersection propety is preserved but quorum avalability property may be violated. So all the processes have to check for quorum avalability without the potentially removed quorum. The remove request will first be send to TOB channel to prevent concurrent removal. After the remove request for quorum $Q'$ delivered from the TOB channel, the process will check $∀ b ∈ \B, ∃ Q ∈ 𝓠 ∖ Q'$, s.t. $Q ∩ B = \emptyset$. If the check pass, $𝓠$ will be updated as $𝓠 ∖ Q'$. If the check fails, the remove request will be dropped. The removal operation will enjoy atomicity thanks to the consistent view for all processes.

\textbf{Add a quoum in DQS}
Adding a quorum is the dual of removing a quorum, which may only endanger quorum intersection property instead of quorum availability property. To add a quorum, a process will first send its add request through a TOB channel to prevent concurrent addition. Upon the delivery of the add request for quorum $Q'$, a well-behaved process check $∀ B ∈ \B, ∀ Q ∈ 𝓠, Q ∩ Q' ∖ B \neq \emptyset$. If the check pass, $𝓠$ will be updated as $𝓠 \cup Q'$. If the check fails, the add request is simply ignored.

\clearpageprime
\subsection{Quorum Sharing}

\begin{comment}
    \begin{figure}[H]
        \centering
        ∈cludegraphics[scale = 0.4]{example2.png}
        \caption{Quorum graph for subjective FBQS example when process 4 lying about quorum slices}
        \label{fig:eg2}
    \end{figure}
\end{comment}

For example, let's assume that the universe contains 5 processes: $𝓟  = \{1, 2, 3, 4, 5\}$ and the Byzantine processes is 4. We have the quorum slices as follow: $\S(1)  = \{\{1, 2\}\}, \S(2) = \{\{2, 3\}, \{2, 4\}, \{2, 5\}\}, \S(3) = \{\{3, 4\}\}, \S(5) = \{\{2, 5\}\}$. Processes 4 lies about its quorum slices: $\S(4)₁  =\{\{1, 4\}\}, \S(4)₂ = \{\{3, 4\}\}, \S(4)_3 = \{\{2, 4\}\},  \S(4)_5 = \{\{4, 5\}\}$. Well-behaved processes construct their individual minimal quorums by sharing slices with each other: $MVQ(1) = \{\{1, 2, 4\}, \{1, 2, 5\}\}, MVQ(2) = \{\{2, 3, 4\}, \{2, 5\}\}$, $MVQ(3) = \{\{2, 3, 4\}\}, MVQ(5) = \{\{2, 5\}\}$. We can see that for processe 1's individual minimal quorum $\{1, 2, 4\}$, we have $2 ∈ \{1, 2, 4\} \wedge ∀ q ∈ 𝓠(2), q \not \subseteq \{1, 2, 4\}$. So we prove that when Byzantine processes lies, we do not have quorum subsumption property across views. The outlive set in the subjective FBQS is $\{1, 2, 5\}$.
            
\begin{figure}
    \caption{Quorum graph for subjective FBQS example when process 4 lying about quorum slices}
    \label{fig:eg2}
    \begin{minipage}{0.2\textwidth}
        \centering
        \begin{tikzpicture}
            \node (top) at (0,0) {$\circled{1}$};
            \node [below of = top, node distance=1.5cm] (bottom) {$\circled{3}$};
            \node [right of = top, node distance=1.5cm] (right) {$\circled{2}$};
            \node [below of = right, node distance=1.5cm] (right bottom) {$\circled{5}$};
            \draw [to-to, line width=0.5pt] (right) -- (right bottom);
            \draw [to-to, line width=0.5pt] (bottom) -- (right);
            \draw [-to, line width=0.5pt] (top) -- (right);
            \draw [-to, line width=0.5pt] (top) -- (right bottom);
        \end{tikzpicture}
    \end{minipage}
    %\hfill
    \begin{minipage}{0.2\textwidth}
        \begin{align*}
            & 𝓠(1) = \{\{1, 2, 4\}, \{1, 2, 5\}\} \\
            & 𝓠(2) = \{\{2, 3, 4\}, \{2, 5\}\} \\
            & 𝓠(3) = \{\{2, 3, 4\}\} \\
            & 𝓠(5) = \{\{2, 5\}\} \\
        \end{align*}
    \end{minipage}
\end{figure}

%Next we show that adding new quorum without coordination can cause violation of quorum intersection property. We reuse the example above as $𝓟₁ = \{1, 2, 3, 4, 5\}, 𝓦₁ = \{1, 2, 3, 5\}, I₁ = \{1, 2, 5\}$. All the quorum slices are the same except that we add $\{5, 6\}$ as a quorum slice of process $5$. We add a new process $6$ with $\S(6) = \{\{5, 6\}\}$. As a consequence,  we have $𝓟₂ = \{5, 6\}, 𝓦₂ = \{5, 6\}, I₂ = \{5, 6\}$. Notice that the two outlive sets internally satisfy the requirements for outliveness in subjective FBQS paper. However, $I₁ \cup I₂ = \{1, 2, 5, 6\}$ does not enjoy quorum intersection property. Since quorum $\{2, 3, 4\} ∩ \{5, 6\} = \emptyset$. From this example we know that even if a well-behaved process choose an outlive process as member of its quorum slice, there is no gurantee that the new system will preserve its outliveness. Our adding protocol prevents such disaster situation and provide all the properties for the new quorum system.

\xl{not needed}

\textbf{Composition Property. \ }

\textbf{Quorum subsumption in other quorum systems}

We argue that quorum subsumption property need to be preserved explicitly and
%Here we notice that in the instaniation paper, authors claimed that 
abstract quorums are not safe abstractions of the quorums in the Stellar Network. 
First of all, we show that when Byzantine processes lie, well-behaved processes may not form complete abstract quorums and do not enjoy quorum subsumption property. Then we show that the set of abstarct quorums is an over-approximation of the observed federated Byzantine quorums. And adding quorums may disable some behavior in the protocol. In other words, a safe protocol works with abstarct quorums may not be safe when working with federated Byzantine quorums.
%The conclusion is based on an observation that all the algorithms presented so far use the notion of quorum only positively. However, we present 
Here we adopt the previous counterexample which disable some behaviors when more quorums are added in the system. For process $2$, we have $𝓠(2) = \{\{2, 3, 4\}, \{2, 5\}\}$. The blocking set of process $2$ is $\textit{Blocking}(2) = \{\{3, 5\}, \{4, 5\}\}$. If we add an abstract quorum $\{1, 2, 4\}$ to process $2$'s quorums, 
the blocking set of process $2$ changes to $\textit{Blocking}(2) = \{\{4, 5\}, \{1, 3, 5\}\}$. 
Before adding the abstarct quorum, receving certain messages from process 3 and 5 is enough to triger next operation. But now with more quorums, process 2 has to wait for additional message from process 1 to proceed. 

Moreover, lemma 17 only makes sure the abstract quorums with only well-behaved members will be observed by well-behaved processes, which does not equal to the statement that after GST all the well-behaved processes will observe all their abstract quorums. For example, process $2$ will never observe its abstract quorum $\{1, 2, 4\}$ when Byzantine process $4$ lies. 

Lemma 15, 16 and 17 is correct. But the inferred conclusion is not. The subtlety lies in the fact that all the abstract quorums form a PBQS while well-behaved processes do not neccessarily observe all the abstract quorums when Byzantine processes lying. By brodcasting inconsistent quorum slices, Byzantine processes can mislead well-behaved processes to have incmoplete abstract quorums, which do not enjoy quorum sharing property across views.

Another false claim appears in section 4.3: the incomplete knowledge about slices will lead to the misunderstanding that certain process set $R$ is not blocking. And this will only remove behaviors in the algorithm. For example, if some process thinks that a process $1$ has the following quorum slices: $\{\{1, 2\}, \{1, 3\}\}$. Then $\{2, 3\}$ is blocking for process $1$. However, if the above information is incomplete, the accurate quorum slices for process $1$ is $\{\{1, 2\}, \{1, 3\}, \{1, 4\}\}$. Then the blocking set for process $1$ changed to $\{2, 3, 4\}$. With the incomplete information, other processes may enable more behaviors rather that removing them. 

\xl{what's the relation between this one and outlive inclusion defined before?}
When Byzantine processes lie about their quorum slices, a weaker version of quorum sharing property holds $∀ v ∈ W, ∃ Q ∈ MVQ(v)$, $Q ⊆ 𝓦 \implies ∀ v' ∈ Q, ∃ Q' ∈ MVQ(v'), Q' ⊆ Q$. Quorum sharing property holds for all the well-behaved processes when their quorums are subsets of well-behaved processes. $∀ v ∈ 𝓦$, if $ ∃ Q ∈ MVQ(v), Q ⊆ 𝓦$, according to the definition of quorum and quorum slices, we have $∀ v' ∈ Q, ∃ \S(v') ⊆ Q$. Then $Q$ is a quorum for process $v'$. Because $Q$ is a subset of well-behaved processes, all the slices stay the same across view. Based on the definition of minimal vertex quorum, $∃ Q' ∈ MVQ(v')$, s.t. $Q' ⊆ Q$. Then we have $∀ v', ∃ Q' ∈ MVQ(v')$, such that $Q' ⊆ Q$.

%Proof for the necessity of quorum sharing property for broadcast. We can prove this by contradiction. Let's assume that quorum sharing property does not stand: $∃ v ∈ 𝓦, v' ∈ I, ∃ Q ∈ MVQ(v) \wedge v' ∈ Q \wedge ∀ Q' ∈ MVQ(v'), Q' \nsubseteq Q$. Let's assume that $v$ delivers a value as a well-behaved process. Acoording to the definition 2 of quorum-based algorithm, there exists an excution in which only $v$ and members of $Q$ take steps and $v$ delivers the value. Then acoording to the totality for outlive processes, $v'$ eventually delivers a value.  

What's the relation of composition property from "How to trust strangers" and our composition property?

In the construction 27, every process use tolerate set to purify some "useless" failure-prone sets of their own. However, the tolerate set is based on the information of actual failure, which is not known to any process in the system. Our leave and join protocols do not rely on such information, which is more feasible in real systems.

The composition property in "How to trust strangers" is fundementally different from our join protocol. The properties preserved in  "How to trust strangers" requires that the failures tolerated in the composed system are also tolerated in the original systems. While our join protocol preserves the inverse of this property: all the failures tolerated in original system are also tolerated in the updated system. This disparate goal leads to divergent composition approaches. In "How to trust strangers" paper, the composed system may potentially tolerate less failures than the original systems. And the composed system's quorums are in the following form: the union of two quorums from two original quorum systems. Then processes in one quorum system has to add some unknown processes from the other quorum system to its own quorums. In our join protocol, the failure-prone sets in the original system are preserved. If the new process's failure assumption does not compliant with the existing one: adding the new quorums and failure assumptions will endanger quorum intersection and availability property, the existing quorum system will reject the compose proposal. However, the process in the intersection of two quorum systems will have the chance to choose new quorums to satisfy quorum sharing property, which minimize the change of quorum in the original system. We use a variant of previous example to demonstrate the differences between two approaches. Assume that we are using symmetric quorum systems: $𝓟₁ = \{1, 2, 3, 4, 5\}, 𝓦₁ = \{1, 2, 3, 5\}, 𝓠₁ = \{\{1, 2, 4\}, \{2, 3, 4\}, \{2, 5\}\}, F₁  = \{\{3, 5\}, \{1, 5\}, \{1, 3, 4\}\}$ and $𝓟₂ = \{5, 6\}, 𝓦₂ = \{5, 6\}, 𝓠₂ = \{\{5, 6\}\}, F₂ = \emptyset$. Then according to construction 14, we have $F_3 = \{1, 3, 4\}, Q_3 = \{2, 5, 6\}$. We can see that adding new process $6$ weakens the tolerated failure sets. And all the processes' quorum are updated to include $\{2, 5, 6\}$.
However, in our join protocol, the new process's join request will be declined because of empty intersection between $\{1, 2, 4\}, \{2, 3, 4\}$ and $\{5, 6\}$.

The relation between quorum sharing and construction 19.
From the proof for quorum sharing's Sufficiency for composition property, we can even weaken the quorum sharing property from all the well-behaved processes's quorums to a subset of the well-behaved process's quorum. Instead of requiring $∀ v ∈ 𝓦, ∀ Q ∈ MVQ(v), ∀ v' ∈ 𝓠, ∃ Q' ∈ MVQ(v') \wedge Q' ⊆ Q$, we can use $∀ v ∈ I₁ ∩ I₂, ∀ v' ∈ 𝓦₁ \cup 𝓦₂$, if $∃ Q' ∈ MVQ(v') \wedge v ∈ Q'$, then $∃ Q ∈ MVQ(v) \wedge Q ⊆ Q'$. The above quorum sharing property is only enforced for outlive processes in the intersection of two outlive sets $I₁ ∩ I₂$. Any well-behaved process who has process $v$ as its quorum member has to contain a individual minimal quorum of process $v$. 

%When we reduce the subjective Byzantine quorum systems to classic quorum systems, we have the weaker quorum sharing property as follow: $∀ v ∈ 𝓦₁ ∩ 𝓦₂, ∀ v' ∈ 𝓦₁ \cup 𝓦₂$, if $∃ Q' ∈ MVQ(v') \wedge v ∈ Q'$, then $∃ Q ∈ MVQ(v) \wedge Q ⊆ Q'$.

The relation between middle processes quorum sharing and composition property.

%Liveness issue. What if a Byzantine process tried to block well-behaved process from entering the system? Does the successes join complete at a well-behaved process push all the related outlive processes complete join, too?
\clearpageprime
\subsection{Examples}

This section includes the federated Byzantine quorum system examples from previous papers. The main purpose is to show the generality of Byzantine quorum graph.

1. Federated byzantine quorum systems: 

Example 1 \& 6: cardinality base quorum system: $\mathcal{U} = \{1, 2, 3, 4\}, \mathcal{B} = \{ \{1\}, \{2\}, \{3\}, \{4\}\}, \mathcal{Q} = \{ \{1, 2, 3\}, \{1, 2, 4\}, \{1, 3, 4\} \{2, 3, 4\}\}$

Example 2 \& 7: $\mathcal{U} = \{1, 2, 3, 4\}, \mathcal{B} = \{\{2\}, \{3, 4\}\}, \mathcal{Q} = \{\{1, 2\}, \{1, 2, 3\}, \{1, 3, 4\}, \{1, 2, 3, 4\}\}$

Example 9: Lying about the quorum slices: $\mathcal{U} = \{1, 2, 3, 4\}, \mathcal{B} = \{\{3\}\}, \mathcal{Q}₁, \mathcal{Q}_4 = \{\{1, 2\}, \{1, 2, 3\},$ $ \{1, 3, 4\}, \{1, 2, 3, 4\}\}, \mathcal{Q}₂ = \{\{1, 2\}, \{1, 2, 3\}, \{1, 2, 3, 4\}\}$

2. Stellar consensus by instantiation: 

$\mathcal{U} ={1, 2, 3}, \mathcal{B} = \{ \emptyset \}, \mathcal{Q} = \{\{1\}, \{1, 2, 3\}, \{2, 3\}, \{1, 2\}, \{1, 3\}\}$, the quorum cluster is $\{2, 3\}$

3. The sum of its parts: analysis of federated byzantine agreement systems:

Almost-Partitioned FBAS: $\mathcal{U} = \{0, 1, 2, 3\}$, 

Casacading failures:

4. Asymmetric byzantine consensus:

$\mathcal{U} = \{1, 2, 3, 4, 5, 6, 7\}, \mathcal{B} = \{4, 5\}, \mathcal{G}_{max} = \{1, 2, 3\}, \mathcal{Q} = \{\{1, 3, 5\}, \{1, 3, 4\}, \{1, 2, 3\}, \{1, 2, 5\},$ $\{1, 2, 4\}, \{2, 3, 5\}, \{2, 3, 4\}, \{2, 4, 5, 6\}, \{1, 2, 6, 7\}, \{1, 2, 3, 4\}, \{1, 2, 4, 5\}, \{1, 3, 4, 5\}, \{2, 3, 4, 5\}, \{1, 2, 3, 5\}\}$

5. Asymmetric Distributed Trust

6. Decentralization in open quorum systems, limitative results for ripple and stellar

$\mathcal{U} ={1, 2, 3, 4, 5, 6}, \mathcal{\{1, 2, 3\}}, \mathcal{Q} = \{\{4, 5, 6\}, \{1, 2, 3, 4, 5, 6\}\}$

7. Deconstructing Stellar Consensus:

Example 2: $\mathcal{U} = \{1, 2, 3, 4 \}, \mathcal{Q} = \{\{1, 2\}, \{2, 3\}, \{3\}, \{4\}\}$

8. Mathematical analysis and algorithms for federated byzantine agreement systems:

Example 2.8: $\mathcal{U} ={1, 2, 3, 4, 5, 6, 7}, \mathcal{B} = \{\{1, 2, 3\}, \{4, 5, 6\}\}, \mathcal{Q} = \{\{1, 2, 3, 7\}, \{4, 5, 6, 7\}, \{7\}\}$
